# Supplementary material for: Improved Algebraic Inverter Modelling for Four-Wire Power Flow Optimization
Source: arXiv:2403.07285 source file (2024-03-12)
Supplement: Supplementary file 1 [file appendix.tex]

\section{next steps/TODOs}
\begin{itemize}
    % \item Fred updates math section to include harmonics everywhere
    \item Fred makes matching figure
    \item Rahmat does detailed literature review, add references immediately in this document
    \item Rahmat sets up a repo for the initial scripts,
    \item implement the initial models just in JuMP, no PMD 4-wire integration planned, only do this if we have time
\end{itemize}

TODOs/questions?
\begin{itemize}
    \item Find more example parameter sets for inverters
    % \item expand lit review with all references
    \item is DQ transform in freq domain correct?
    \item model inverter output filter?
    % \item skip harmonic modelling?
    \item study \cite{Cunha2021} in detail, seems to be very good
    % \item what is the real contribution of NREL/Jose Daniel Lara? \cite{lara2023revisiting}
    \item Grid-following inverters may still have positive sequence current control to minimize ripple on the dc bus
    % \item consider asking Matthew Deakin to collaborate by mid August [to be revisited]
\end{itemize}

\begin{itemize}
    \item Data-driven modelling using Splines. Discuss other loss models?
\end{itemize}

{\color{blue}
TODOs
\begin{itemize}
    \item describe also how OpenDSS /PMD does it (three-wire, grounded neutral, with some loss model), so we can set up a comparison (crucial for publishing)
    \item add discussion of the GridLab-D approach as well!
    % \item review of harmonic load models + harmonic inverter models (interaction with control bandwith. Starting point is Brunoro et al 
    % \item come up with harmonic math
    \item come up with best possible approximation for active filters (combine unbalance operation, losses, but otherwise no active power consumption/injection)
    \item Add positive and zero sequence model descriptions.
    \item Add additional equations that could help short circuit studies?
\end{itemize}
}

\subsection{Inverter Model in PMD / OpenDSS (three-wire)}
% \subsection{Nonlinear Multi-Conductor Converter Model}
The complex power flow from the grid into the converter $\indexconverter$, through conductor $\indexconductor$, at time $\indextime$, is given by,
\begin{IEEEeqnarray}{C}
\Scpt = \Pcpt + \imag \Qcpt. \label{eq_power}
\end{IEEEeqnarray}
We define the set of conductors (phases), $\indexconductor \in \setconductor$.  
This power flow is subject to a per-conductor apparent power flow rating $\Scratingp$ and current limit $\Icratingp$ and a time-dependent operational status parameter $\statusct \in \{0,1\}$,
\begin{IEEEeqnarray}{C}
  |\Scpt|^2  \leq (\statusct \cdot \Scratingp)^2, \quad
  |\Icpt|  \leq \statusct \cdot \Icratingp \label{eq_current_power_limits}
      \end{IEEEeqnarray}
  The relationship between power, current and voltage magnitude is given by,
\begin{IEEEeqnarray}{C}
     |\Scpt|^2 = |\Uipt|^2 |\Icpt|^2. \label{eq_complex_power_def}
     \end{IEEEeqnarray}
Combining these properties, the converter's power balance and losses are defined as,
\begin{IEEEeqnarray}{C}
 \!\!\!\!\!\!\underbrace{ \sum_{\indexconductor \in \setconductor}  \Scpt }_{\text{grid side power}} \!+ \!\!\!\!\!\!\underbrace{\Pstor}_{\text{energy buffer}} \!\!\! =  \!\!\! \underbrace{\imag \Qint}_{\text{reactive source}} \!\!\! + \!\! \underbrace{\Sext}_{\text{other flow}} \!\!\!+\!\!  \underbrace{\sum_{\indexconductor \in \setconductor} \Zcp |\Icpt|^2.}_{\text{copper loss}} \label{eq_balance_loss}
\end{IEEEeqnarray}
This equation is composed of five components (left to right):
\begin{itemize}
    \item the complex power flow supplied through all converter's conductors $\Scpt$;  
    \item the storage subsystem active power $\Pstor$;  
    \item a variable $\Qint$ that represents the converter's ability to control the generation and/or absorption of reactive power;
    \item the user-defined complex power $\Sext$;  
    \item copper losses proportional to internal impedance $\Zcp$ and current magnitude $\Icpt$ squared.
\end{itemize}
Note that the inclusion of a copper loss term, due to its quadratic nature, incentivizes charging and discharging slowly over time, as well as avoiding unnecessary reactive power injection or consumption.  This has an added benefit of avoiding degeneracy issues related to multiple reactive power sources and sinks on a single node.  If reactive power is absorbed or generated in the inverter, the reactive power in \eqref{eq_balance_loss} remains balanced through variable $\Qint$.  

The $\Sext$ parameter often represents unavoidable losses that are incurred while the system is idle, but it can also be used to capture a wide variety of exogenous energy sinks or sources. Examples of exogenous flows are, self-discharge in a battery and water flow into the upper reservoir of a pumped hydro plant.

% \subsection{Harmonic models}
% TODO: review of harmonic load models + harmonic inverter models (interaction with control bandwith. Starting point is Brunoro et al 

% Inverters, due to their modulated power electronic switches also may produce certain harmonics. Furthermore, the interaction of inverters with harmonics already present in the grid isn't well-studied in steady-state. 
% A grid-connected inverter may be affected by harmonics produced from the grid along with the nonlinear characteristic of the PWM unit. 
% Harmonics are normally modeled in the time domain, which poses a non-trivial challenge to study these effects in frequency-domain optimization models. 
% % Fourier transform is a useful technique for harmonics modelling and LCL filter is commonly used to attenuate the inverter harmonics. 
% %

% In addition, inverters are the technology underlying active harmonic filters, where the control loops are designed to inject harmonic currents in anti-phase to off-set the harmonics present in the network. The representation of harmonics and such control laws in the context of four-wire OPF is an emerging topic that warrants further research \cite{GETH2022108604}.
% The abilities of different types of inverters to inject and absorb harmonics is not well established.

The above definitions can be applied to current unbalance:
\begin{IEEEeqnarray}{C}
    \label{eq:IUF}
    \%IUF = I_{i,2} / I_{i,1},
    \\
    \label{eq:IUF2}
    \%IUF_2 = I_{i,2},
    \\
    \label{eq:PIUR}
    \%PIUR = \max_p \big(I_{i,p} - \frac{1}{3} \sum\nolimits_p I_{i,p}\big) / \big(\frac{1}{3} \sum\nolimits_p I_{i,p}\big).
\end{IEEEeqnarray}

Definition of unbalance can also be extended to active and reactive power as
\begin{IEEEeqnarray}{C}
    \label{eq:PPUR}
    % \%PPUR = \frac{\max_p (P_{i,pp} - \frac{1}{3} \sum_p P_{i,pp})}{\frac{1}{3} \sum_p P_{i,pp}},
    \%PPUR = \max_{p\in \mathcal{P}} \big|P_{i,p} - \frac{1}{3} \sum\nolimits_p P_{i,p}\big| /\big( \frac{1}{3} \sum\nolimits_p P_{i,p} \big)
    \\
    \label{eq:PQUR}
    \%PQUR = \max_{p\in \mathcal{P}} \big|Q_{i,p} - \frac{1}{3} \sum\nolimits_p Q_{i,p} \big| / \big( \frac{1}{3} \sum\nolimits_p Q_{i,p} \big)
\end{IEEEeqnarray}
